# Supplementary material for: Sounds and hydrodynamics of polar active fluids
Source: arXiv:1810.00585 ancillary file (2018-10-01)
Supplement: Supplementary file 1 [file Geyer2017SIV2.pdf]

# Supplementary Materials:
# Sounds and hydrodynamics of polar active liquids

Delphine Geyer,[1] Alexandre Morin,[1] and Denis Bartolo[1]

[1] *Univ Lyon, ENS de Lyon, Univ Claude Bernard Lyon 1, CNRS, Laboratoire de Physique, F-69342 Lyon, France*

## CONTENTS

Supplementary videos legends 2

Supplementary Note 1 : Giant density fluctuations 3
1. Colloidal roller liquids display giant density fluctuations 3
2. Critical discussion of the results published in [1] 4

Supplementary Note 2: Hydrodynamic theory of polar active liquids 4
1. Toner and Tu hydrodynamics 4
2. Linear fluctuations 5
3. Dispersion relations of the slow modes 6
4. Speed of sound 6
5. Sound-wave damping and measurement of the orientational-elasticity constants 6
    5.1 . Transverse waves: $\theta = \pi/2$ 7
    5.2 . Oblique waves: $\theta = \pi/4$ 7
6. Colloidal-roller hydrodynamics 8
    6.1 . Microscopic dynamics 8
    6.2 . Kinetic theory of the polar-liquid phase 9
    6.3 . Hydrodynamic theory 10
    6.4 . Critical discussion of the kinetic theory 10

Supplementary Note 3 : Independence of the material parameters on the channel geometry 12

Experimental setup 13

Supplementary References 13

## SUPPLEMENTARY VIDEOS LEGENDS

*a. Supplementary video 1.* An active polar liquid composed of $\sim 3\times10^6$ colloidal rollers flows in a microfluidic racetrack. We show the trajectories of five particles, and the instantaneous orientation of their velocity (black arrows). They fluctuate around the average direction of the emergent flow. The polar liquid does not move like a rigid body, the particles rearrange. The area fraction of the colloids is $\rho_0 = 0.11$. Colloid diameter: 4,8 $\mu$m. Field amplitude: $E_0 = 2\,\mathrm{V}/\mu\mathrm{m}$. Movie recorded at 500 fps, played at 30 fps.

*b. Supplementary video 2.* An active polar liquid composed of $\sim 3\times10^6$ colloids flows in a microfluidic racetrack. The color indicates the magnitude of the velocity-component transverse to the mean flow. Blue particles are moving up, red particles are moving down. Transverse velocity fluctuations propagate through the polar liquid. The area fraction of the colloids is $\rho_0$=0,11. Colloid diameter: 4,8 $\mu$m. Field amplitude: $\mathrm{E}_0$=2 V/$\mu$m. Movie recorded at 500 fps, played at 20 fps.

*c. Supplementary video 3.* Density field of a polar liquid flowing in a microfluidic racetrack. The density field is defined in the Voronoi cells centred on the particles. The color of the cells indicates the inverse of the cell area, and therefore corresponds to the local colloid density. The density fluctuations propagate in different directions when the polar liquid flows. The area fraction of the colloids is $\rho_0$=0,11. Colloid diameter: 4,8 $\mu$m. Field amplitude: $\mathrm{E}_0$=2 V/$\mu$m. Movie recorded at 500 fps, played at 20 fps.

# SUPPLEMENTARY NOTE 1 : GIANT DENSITY FLUCTUATIONS

## 1. Colloidal roller liquids display giant density fluctuations

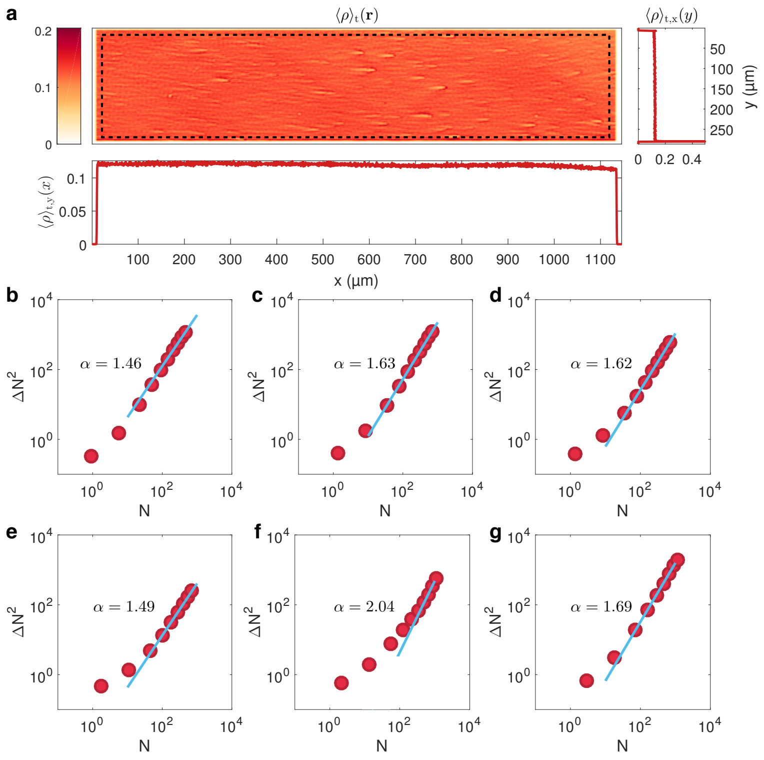


Supplementary Figure 1. **Giant number fluctuations.** **a**, Time averaged density field of a polar liquid with an average area fraction of $\rho_0 = 0.12$. The color on the heat map indicates the local value of the time averaged area fraction. Dashed line: region where the number fluctuations are computed.The corresponding $x$ and $y$ averaged density profiles are plotted respectively below and on the right hand side of the density plot. **b**-g, Number fluctuations $\Delta N^2$ plotted versus the average number of particles $N$ for average area fractions of $\rho_0 = 0.119$, $\rho_0 = 0.182$, $\rho_0 = 0.183$, $\rho_0 = 0.236$, $\rho_0 = 0.300$ and , $\rho_0 = 0.397$. Solid line bets power law fit and value of the fitted power law.

Giant number fluctuations are one of the most remarkable features of active liquids with uniaxial orientational order [4, 5]. This phenomenon has been consistently reported for a variety of experimental systems ranging from shaken grains, to bacteria suspensions and motility assays, see [11] for a comprehensive list and a critical assessment of the available measurements and simulations. Even though there is no doubt about the existence of giant number fluctuations in ordered liquids assembled from motile particles, their measurement is extremely delicate as subject to a number of possible artefacts. The determination of the exact scaling law relating the fluctuations, $\Delta N^2(\ell)$, of the number of particles in a box of size $\ell$ to the average number $N(\ell)$ goes beyond the scope of this letter. We however unambiguously establish that the number fluctuations in polar active liquids assembled from colloidal rollers are giant. Performing measurements on six different polar liquids of average packing fractions comprised between $\rho = 0.12$ and $\rho = 0.39$, we find $\Delta N^2 \sim N^\alpha$ with $1.46 < \alpha < 2.04$, as detailed below.

Number fluctuations are all measured in steady state, and in the most homogeneous region of our device. The homogeneity of the polar liquid was checked by measuring the time average density field in the entire observation window as illustrated in Fig. 1a. Number fluctuations are computed only in regions of space where the static spatial heterogeneities are less than 10%. The statistics is accumulated over 5,000 frames. The number of particules is counted in square boxes of increasing length. The results of the number statistics are shown separately for each experiment in Figs. 1b to 1g. A power law fit of the data is performed for values of $N$ larger than 10. The values of the $\alpha$ exponent are systematically found to be larger than 1 establishing the existence of giant number fluctuations in all roller fluids. Importantly, we stress that this anomalous scaling does not originate from the static heterogeneities of the density field. The static fluctuations of $\Delta N^2$ are found to be between one and two orders of magnitude smaller than the dynamical fluctuations.

The unambiguous existence of giant number fluctuations calls for a critical discussion of the conflicting measurement reported in [1].

### 2. Critical discussion of the results published in [1]

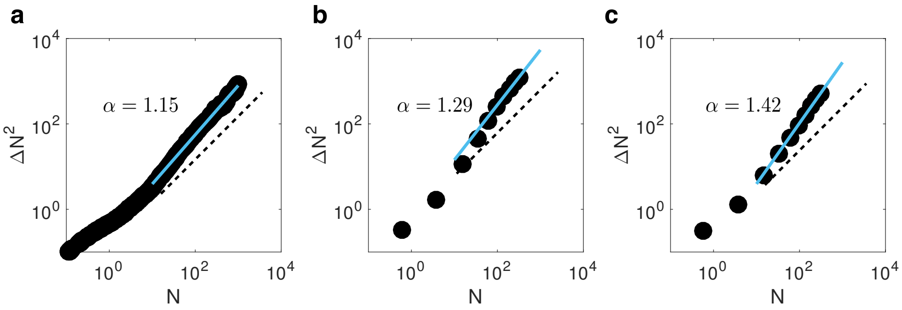


Supplementary Figure 2. **Giant number fluctuations, comparison with the results from [1].** **a**, Number fluctuations $\Delta N^2$ plotted versus the average number of particles $N$. Average area fractions of $\rho_0 = 0.095$. These data correspond to that of Fig. 4c in [1]. Dashed line: normal fluctuations $\Delta N^2 \sim N$. Solid line: best power law fit giving $\Delta N^2 \sim N^\alpha$ with $\alpha = 1.15$. **b** and **c** Number fluctuations $\Delta N^2$ plotted versus the average number of particles $N$ measured from two different movies including Supplementary Video 4 from [1] (average area fractions of $\rho_0 = 0.18$). The number fluctuations are found to be giant with exponents $\alpha = 1.29$ and $\alpha = 1.42$.

In [1] using the same experimental system (aside from minor technical differences: slightly different AOT salt concentration, different gap between the electrodes and use of another insulating layer to confine the colloids), polar liquids assembled from colloidal rollers were reported to display normal density fluctuations. This conclusion was erroneous and certainly due to a poorer statistics. The results reported in Fig. 4c from [1] are reproduced in Fig. 2a below. The quality of the data does not make it possible to distinguish between any value of $\alpha$ comprised between 1 (dashed line) and 1.2 (Solid line and best power-law fit).

We have also analysed two additional experiments published in [1], including the polar-liquid movie presented in Supplementary Video 4 from [1] and corresponding to $\rho_0 = 0.18$. The number fluctuations computed over the entire ensemble of available frames using the same algorithm as in the present study are plotted in Figs. 1b and 1c. Again the number fluctuations significantly deviates from a normal behavior. The values of the $\alpha$ exponents are consistent with that found in the present study. From this complementary analysis, we rectify the conclusion drawn in [1] and conclude that colloidal roller fluids display the giant number fluctuations typical to all uniaxial active liquids.

We conclude this critical discussion, by addressing the theoretical explanation put forward in [1] to justify the apparent lack of anomalous number fluctuations. The microscopic theory of roller interactions includes long range hydrodynamic interactions that were predicted to damp splay and density fluctuations at long wave lengths. Our speed of sound measurements indicate that these long-range interactions do not have any impact on the roller dynamics at the scale of our experiments. As a matter of fact, this damping term would result in a dispersion relation scaling as $\omega \sim$ const as $q \to 0$. This prediction is not supported by our experimental measurements, Fig. 2 in the main text. The reason for this discrepancy is very likely to be due to the very small magnitude of the long-range hydrodynamic interactions having a strength set by the ratio $a/H = 2 \times 10^{-2}$ between the colloid radius $a$ and the distance between the two electrodes $H$. Probing the potential impact of these hydrodynamic interactions would require performing experiments at much larger scales out of reach of our current setup.

## SUPPLEMENTARY NOTE 2: HYDRODYNAMIC THEORY OF POLAR ACTIVE LIQUIDS

### 1. Toner and Tu hydrodynamics

We recall below the hydrodynamic description of polar flocks, also termed polar active liquids, as first introduced by Toner and Tu in [3] and reviewed in [4, 5]. These active materials are associated with two hydrodynamic fields: the liquid density $\rho(\mathbf{r}, t)$, and the local velocity field $\mathbf{v}(\mathbf{r}, t)$. $\rho(\mathbf{r}, t)$ is a slow variable because particle number is conserved, while $\mathbf{v}(\mathbf{r}, t)$ is a slow variable only in the polar-liquid phase where rotational symmetry is spontaneously

broken. As a matter of fact, we are dealing here with an instance of dry active matter where momentum is not conserved [5]. In the case of active colloids propelling on a substrate, the solid surface acts as a momentum sink. Toner and Tu constructed a set of phenomenological equations of motion using only symmetry and conservation principles. Since then, these equations have been confirmed by kinetic theories constructed both from minimalistic and realistic microscopic models [1, 6, 7]. For a 2D active liquid, in their most general form, Toner and Tu equations read:

$$\partial_t \rho + \nabla \cdot (\mathbf{v}\rho) = D\Delta\rho, \tag{1}$$

and,

$$\begin{aligned} \partial_t \mathbf{v} + \lambda_1(\mathbf{v}\cdot\nabla)\mathbf{v} + \lambda_2(\nabla\cdot\mathbf{v})\mathbf{v} + \lambda_3\nabla(|\mathbf{v}|^2) = {}& a_2\mathbf{v} - a_4|\mathbf{v}|^2\mathbf{v} - \sigma_1\nabla\rho - \sigma_2\left(\mathbf{v}\cdot\nabla\rho\right)\mathbf{v} \\ & + D_B\nabla\left(\nabla\cdot\mathbf{v}\right) + D_T\nabla^2\mathbf{v} + D_2\left(\mathbf{v}\cdot\nabla\right)^2\mathbf{v} \\ & + D_{\rho 1}\Delta\rho\mathbf{v} + D_{\rho 2}\left[\left(\mathbf{v}\cdot\nabla\right)^2\rho\right]\mathbf{v} + D_{\rho 3}\nabla\left(\mathbf{v}\cdot\nabla\rho\right). \end{aligned} \tag{2}$$

Eqs. (1) and (2) include 14 unknown materials constants which a priori all depend on $\rho$. Before recalling the physical meaning of these lengthy equations, we note that the last three terms were neglected in [3]. We keep them here as they are allowed by symmetry and are of the same order in a gradient expansion. The $\lambda_i$s are all convective coefficients. $\lambda_2 = \lambda_3 = 0$ and $\lambda_1 = 1$ is a normal, passive fluid. The $a_2$ and $a_4$ terms are the usual Ginsburg Landau term allowing for spontaneous symmetry breaking. Their ratio sets the magnitude of the mean flow speed in the ordered phase. The $D_\mathrm{B}$, $D_\mathrm{T}$ and $D_2$ terms in Eq. (2) are the anisotropic elastic (Frank) constants of this broken symmetry fluid. The $D_\rho$s couple density and elastic deformations. $D$ is the translation diffusion of the active particles which we neglect below.

### 2. Linear fluctuations

We are interested in describing the linear fluctuations of the density and velocity fields in a homogeneous polar liquid of average density $\rho = \rho_0 + \delta\rho$ and velocity $\mathbf{v}(\mathbf{r},t) = [u_0 + u(\mathbf{r},t)]\,\hat{\mathbf{x}} + v(\mathbf{r},t)\hat{\mathbf{y}}$. Once linearized around this steady state, the three equations of motion take the form:

$$\partial_t\rho + \rho_0\left(\partial_x u + \partial_y v\right) + u_0\partial_x\rho = 0, \tag{3}$$

$$\begin{aligned} \partial_t u + \lambda_1 u_0\partial_x u + \lambda_2 u_0\left(\partial_x u + \partial_y v\right) + 2\lambda_3 u_0\partial_x u = {}& -2a_4u_0^2u - \sigma\partial_x\rho \\ & + (D_T + D_B + D_2u_0^2)\partial_{xx}u + D_B\partial_{xy}v + D_\mathrm{T}\partial_{yy}u \\ & + u_0(D_{\rho 1} + D_{\rho 3} + u_0^2D_{\rho 2})\partial_{xx}\rho + D_{\rho 1}u_0\partial_{yy}v, \end{aligned} \tag{4}$$

$$\begin{aligned} \partial_t v + \lambda_1 u_0\partial_x v + 2\lambda_3 u_0\partial_y u = {}& -\sigma\partial_y\rho + D_{\rho 3}u_0\partial_{xy}\rho \\ & + (D_T + D_B)\partial_{yy}v + D_B\partial_{xy}u + (D_2u_0^2 + D_\mathrm{T})\partial_{xx}v, \end{aligned} \tag{5}$$

We have also ignored the anisotropy of the liquid compressibility by setting $\sigma_2 = 0$ and noted $\sigma_1 = \sigma$ as it will play no role in all that follows. Eq. (4) indicates that longitudinal velocity fluctuations relax in a finite time of the order $1/(2a_4u_0^2)$. In the hydrodynamic limit the variations of $u$ are therefore slaved to $\rho$ and $v$. Focusing on time scales larger than $1/(2a_4u_0^2)$, and length scales larger than $\lambda_1/(2a_4u_0)$, Eq. (4) readily simplifies into:

$$u = -\frac{\sigma}{2a_4u_0^2}\partial_x\rho + \mathcal{O}(\nabla^2). \tag{6}$$

This relation is verified in our experiments, see Fig. 3b in the main text. Plugging Eq. (6) into Eqs. (3) and (5), the linear dynamics of the only two slow modes take the much simpler form:

$$\partial_t\rho + \rho_0\left(\partial_y v\right) + u_0\partial_x\rho = D'\partial_x^2\rho \tag{7}$$

$$\partial_t v + \lambda_1 u_0\partial_x v = -\sigma\partial_y\rho + D_\perp\partial_y^2 v + D_\parallel\partial_x^2 v + u_0D_\rho\partial_{xy}^2\rho \tag{8}$$

where,

$$D_\perp = D_T + D_B \tag{9}$$

$$D_\parallel = D_2u_0^2 + D_\mathrm{T} \tag{10}$$

$$D_\rho = D_{\rho_3} - \frac{\lambda_3\sigma}{a_4u_0^2} \tag{11}$$

$$D' = \frac{\sigma\rho_0}{2a_4u_0^2} \tag{12}$$

While $D'$ is measured from the linear relation between density and longitudinal-velocity fluctuations, Fig. 3b, a more careful analysis of the fluctuation spectra is required to measure the values of the five other material constant characterizing the linear hydrodynamics of the polar fluid: $\lambda_1$, $\sigma$, $D_\perp$, $D_\parallel$, and $D_\rho$.

### 3. Dispersion relations of the slow modes

Let us look for for plane-wave solutions of the two linear equations defined by Eqs. (40) and (41). Writing the wave amplitudes $\rho(\mathbf{q},\omega)$ and $v(\mathbf{q},\omega)$, where $\omega$ is the frequency and $\mathbf{q} = q(\cos\theta, \sin\theta)$ is the wave vector, we find that they obey the matrix equation:

$$i\omega \begin{bmatrix}\rho(\mathbf{q},\omega)\\ v(\mathbf{q},\omega)\end{bmatrix} = \mathbf{M}\cdot \begin{bmatrix}\rho(\mathbf{q},\omega)\\ v(\mathbf{q},\omega)\end{bmatrix}. \tag{13}$$

The response matrix $\mathbf{M}$ is defined as $\mathbf{M} = iq\mathbf{C} - q^2\mathbf{D}$, where

$$\mathbf{C} = \begin{pmatrix} u_0\cos(\theta) & \rho_0\sin(\theta)\\ \sigma\sin(\theta) & \lambda_1 u_0\cos(\theta)\end{pmatrix}, \tag{14}$$

and

$$\mathbf{D} = \begin{pmatrix} D'\cos^2\theta & 0\\ \frac{1}{2}u_0 D_\rho\sin(2\theta) & D_\parallel\cos^2(\theta) + D_\perp\sin^2(\theta)\end{pmatrix}. \tag{15}$$

The eigenvectors of the linear system defined by Eq. (13) are mixed modes coupling density and transverse velocity fluctuations. Their dispersion relations are defined by the eigenvalues $\omega_\pm(q,\theta)$ of $\mathbf{M}(\mathbf{q})$ which take a simple form in the limit of small wavevectors:

$$\omega_\pm(q,\theta) = \left[c_\pm(\theta)q + \mathcal{O}(q^3)\right] + i\Delta\omega_\pm(q,\theta). \tag{16}$$

The associated eigenmodes correspond to non-dispersive plane waves propagating with a phase velocity $c_\pm$ and attenuated over a time $2\pi/(\Delta\omega_\pm)$.

### 4. Speed of sound

Unlike sound waves in isotropic passive liquids, $c_\pm$ depends on the direction of propagation $\theta$. As predicted first by Toner and Tu [3], we find:

$$2c_\pm(\theta) = (1+\lambda_1)\, u_0\cos\theta \pm \sqrt{(\lambda_1 - 1)^2\, u_0^2\cos^2\theta + 4\sigma\rho_0\sin^2\theta}. \tag{17}$$

The non-monotonic angular variations of the speed of sound are in excellent agreement with our experimental findings, see Figure 2 g,h,i in the main text. Analysing the angular variations of the speed of sound, we infer both the convective coefficient $\lambda_1$ and the compressibility $\sigma$, see Fig. 3c. As thoroughly explained below, measuring the orientational elasticity of the polar liquid requires inspecting the damping dynamics, or equivalently the spectral width of the density and velocity fluctuations.

### 5. Sound-wave damping and measurement of the orientational-elasticity constants

Let us consider the linear response of the polar liquid to a random white noise $\boldsymbol{\xi} = (\xi_\rho(\mathbf{r},t), \xi_v(\mathbf{r},t))$. $\xi_\rho$ is conserved while $\xi_v$ is a non conserved random force field acting respectively on $\rho$ and $v$. In Fourier space the stochastic equations of motion are:

$$i\omega \begin{bmatrix}\rho(\mathbf{q},\omega)\\ v(\mathbf{q},\omega)\end{bmatrix} = \mathbf{M}\cdot \begin{bmatrix}\rho(\mathbf{q},\omega)\\ v(\mathbf{q},\omega)\end{bmatrix} + \boldsymbol{\xi}(\mathbf{q},\omega). \tag{18}$$

The power spectra of both $\rho$ and $v$ are easily computed from Eq. (18) and take the same functional form:

$$|v(\mathbf{q},\omega)|^2 = \frac{\alpha_+}{(\omega - c_+ q)^2 + \Delta\omega_+^2} + \frac{\alpha_-}{(\omega - c_- q)^2 + \Delta\omega_-^2} \tag{19}$$

where the noise variance sets the values of the amplitude factors $\alpha_\pm$ which are irrelevant to all that follows. The velocity spectrum is the sum of two Lorentzian functions peaked along the dispersion relations $\omega = c_\pm(\theta)q$. This low-$q$ theory accurately predicts the non-dispersive part of the dispersion relation, but obviously fails in describing wave dispersion at short wave lengths, Figs. 2d,e,f. The spectral width $\Delta\omega_\pm$ is computed from Eq. (13):

$$\Delta\omega_\pm(q,\theta) = \frac{q^2}{4}\left[-(D' + D_\perp + D_\parallel) - (D' + D_\parallel - D_\perp)\cos(2\theta) \pm D_\rho u_0\sqrt{\frac{\rho_0}{\sigma}}\sin(2\theta)\right] + \mathcal{O}(q^3) \tag{20}$$

This expression is rather complex, yet it is clear that the spectral width of the sound modes is set by the elastic constants of the broken symmetry fluid. Their values and their variations with the average fluid density are easily computed when inspecting the two cases corresponding to $\theta = \pi/2$ and $\theta = \pi/4$.

### 5.1 . *Transverse waves: $\theta = \pi/2$*

The case of sound waves propagating along the transverse direction $\theta = \pi/2$ is straightforward. The two dispersion relations are symmetric, see Fig. 2e, the two speeds of sound are opposite, $c_\pm(\pi/2) = \pm\sqrt{\sigma\rho_0}$, and their spectral width grows quadratically with $q^2$ as expected:

$$\Delta\omega_\pm(\pi/2) = \frac{1}{2}D_\perp q^2. \tag{21}$$

High-$q$ distortions are more effectively suppressed by the alignment interactions between the active particles, or equivalently by orientational elasticity. Fitting the variations of $\Delta\omega_\pm(\pi/2)$ by a quadratic function provides a direct measurement of $D_\perp$. Repeating the same procedure for all densities we find that $D_\perp$ increases lienarly with $\rho_0$. The denser the polar liquid, the stiffer.

### 5.2 . *Oblique waves: $\theta = \pi/4$*

Repeating the same analysis at $\theta = \pi/4$, we find that the two sound modes propagate at $c_\pm(\pi/4) = \frac{1}{\sqrt{2}}\left(u_0 \pm \sqrt{\sigma\rho_0}\right)$. The spectral width of the two modes grows again as $q^2$, and are related to the elastic constants by

$$\Delta\omega_+\left(\frac{\pi}{4}\right) + \Delta\omega_-\left(\frac{\pi}{4}\right) = \left(D_\perp + D_\parallel + D'\right)q^2, \tag{22}$$

and

$$\Delta\omega_+\left(\frac{\pi}{4}\right) - \Delta\omega_-\left(\frac{\pi}{4}\right) = \frac{\rho_0 D_\rho u_0}{\sqrt{\sigma\rho_0}}q^2. \tag{23}$$

Fitting $\Delta\omega_+\left(\frac{\pi}{4}\right) + \Delta\omega_-\left(\frac{\pi}{4}\right)$ by a quadratic function of the wave vector provides a direct measurement of the average elastic constant $\left(D_\perp + D_\parallel + D'\right)$, see Eq. (22). As shown in the main text, we find a value 4 orders of magitude larger than that of $D'$ which can therefore be neglected. As $D_\perp$ is known from the previous analysis at $\theta = \pi/2$, $D_\parallel$ is readily deduced from the quadratic fit of $\Delta\omega_+\left(\frac{\pi}{4}\right) + \Delta\omega_-\left(\frac{\pi}{4}\right)$.

The last material constant to be determined is $D_\rho$. In principle, it could be measured by fitting $\Delta\omega_+\left(\frac{\pi}{4}\right) - \Delta\omega_-\left(\frac{\pi}{4}\right)$ by a quadratic function of $q$, as both $u_0$ and $\sigma$ were already measured independently (from velocity and sound speed measurements, see Fig. 3 and Eq. (17)). In the specific case of our colloidal-roller experiments, the precision of our measurements of $\Delta\omega_\pm$ prevents us from determining $D_\parallel$. Nonetheless, this last material constant can be estimated exploiting our quantitative understanding of the colloidal-roller interactions as explained.

## 6. Colloidal-roller hydrodynamics

### *6.1 . Microscopic dynamics*

We briefly recall the kinetic-theory framework used to derive of the Toner and Tu equations for the polar-liquid phase of colloidal rollers. In [1], starting from the Maxwell and Stokes equations, and after lengthy algebra, we showed that the rollers propel at constant speed, $\nu_0$, and interact via their orientational degree of freedom only. Noting $\mathbf{r}_i$ the position of their center of mass, and $\theta_i$ the orientation of their velocity $\boldsymbol{\nu}_i(t) = \nu_0(\cos\theta_i, \sin\theta_i)$, their translational and angular dynamics can be recast into the compact form:

$$\partial_t \mathbf{r}_i(t) = \nu_0 \hat{\boldsymbol{\nu}}_i, \tag{24}$$

and

$$\partial_t \theta_i(t) = -\partial_{\theta_i} \sum_{j\neq i} \mathcal{H}(\mathbf{r}_i - \mathbf{r}_j; \theta_i, \theta_j) + \sqrt{2D_{\mathrm{R}}}\xi_i(t) \tag{25}$$

where the $\xi_i$ are uncorrelated Gaussian white noises of unit variance, and where the effective interaction potential $\mathcal{H}$ is given by

$$\mathcal{H}(\mathbf{r}_i - \mathbf{r}_j; \theta_i, \theta_j) = A(r)\hat{\boldsymbol{\nu}}_i \cdot \hat{\boldsymbol{\nu}}_j + B(r)\hat{\boldsymbol{\nu}}_i \cdot \mathbf{r} + C(r)\hat{\boldsymbol{\nu}}_j \cdot (2\hat{\mathbf{r}}\hat{\mathbf{r}} - \mathbb{I}) \cdot \hat{\boldsymbol{\nu}}_i. \tag{26}$$

This functional form turns out to be very generic [8] and corresponds to the first three terms of a systematic multipolar expansion of the angular interactions. In the specifc case of interacting rollers the three kernerls $A(r)$, $B(r)$ and $C(r)$ can be approximated within a far field approximation for the hydrodynamic and electrostatic interactions:

$$A(r) = A_1 \left(\frac{a}{r}\right)^3 \Theta(r) + A_2 \left(\frac{a}{r}\right)^5 \Theta(r), \tag{27}$$

$$B(r) = B_1 \left(\frac{a}{r}\right)^4 \Theta(r), \tag{28}$$

$$C(r) = C_1 \left(\frac{a}{r}\right)^3 \Theta(r) + C_2 \left(\frac{a}{r}\right)^5 \Theta(r) + C_3 \left(\frac{a}{r}\right)^2. \tag{29}$$

The $A$ term in Eq. (26) is akin to a ferromagnetic coupling, and stems both from hydrodynamic ($A_1$) and electrostatic interactions ($A_2$). The $B$ term is a repelling torque that originates from the electrostatic interactions between the electrostatic dipoles formed by the surface charges of the rollers. Finally, the $C$ term promotes alignment of the roller $i$ along a dipolar field centered on roller $j$. This term has three different origins. The $C_1$ and $C_2$ terms have the same microscopic origin as $A_1$ and $A_2$, while $C_3$ stems from the finite size of the rollers and vertical confinement which altogether result in genuinely long-range interactions. All other interactions are indeed screened over a distance set by the channel height $H$. For the sake of simplicity, we approximate the screening function $\Theta(r)$ by a step function $\Theta(r) = 1$ if $r \leq H/\pi$ and $\Theta(r) = 0$ otherwise.

All the scalar coefficients in Eqs. (27), (28) and (29) have units of inverse time scales, and are all of the order of the so-called Maxwell relaxation rate $\tau^{-1} \sim 3\,\mathrm{kHz}$ [1, 9]. Rotational diffusion was measured from the exponential decay of the correlations of the roller orientation in the gas phase [1, 2, 10]. Within our experimental conditions, we find [2]:

$$A_1 = A_2 = B_1 = C_1 \sim \tau^{-1} \tag{30}$$

$$C_2 \sim 1.7\tau^{-1} \tag{31}$$

$$C_3 \sim (4.5 \times 10^{-2})\tau^{-1} \tag{32}$$

$$D_{\mathrm{R}} \sim 3\,\mathrm{s}^{-1} \tag{33}$$

As $C_3$ is a thousand times smaller that all the other interaction strengths, we henceforth neglect this contribution to Eq. (29). This simplification is further supported by the very good agreement between our measurements and our hydrodynamic theory described in the main text. The last two parameters needed to fully specify the dynamics of the rollers are the screening distance $H = 110\,\mu\mathrm{m}$, and the roller speed $\nu_0$. Our simplified model predicts a constant roller speed at all densities. To go beyond this approximation we measured the variations of $\nu_0$ with the average density $\rho_0$ and use this relation as a phenomenological law Fig. 3.

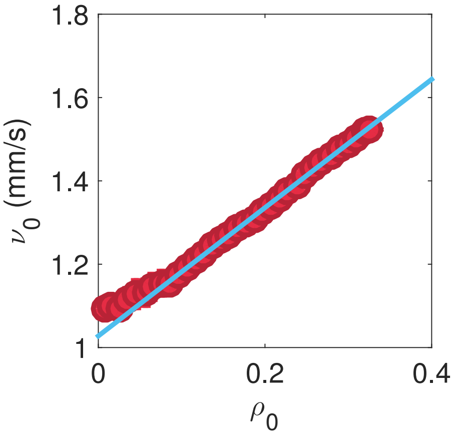


Supplementary Figure 3. **Roller speed.** Red dots: Variations of the roller speed with the roller area fraction $\rho_0$. Blue line: best linear fit.

### *6.2 . Kinetic theory of the polar-liquid phase*

We now outline the construction of the hydrodynamic equations for the density and velocity fields in the polar-liquid phase. We use here a conventional kinetic-theory framework reviewed e.g. in [5]. We first write a conservation equation for the one-point distribution function $\psi(\mathbf{r},\theta,t)$, viz the probability to find a particle at position $\mathbf{r}$ with an orientation $\theta$:

$$\partial_t\psi(\mathbf{r},\theta,t) + \nu_0\hat{\boldsymbol{\nu}}\cdot\nabla\psi(\mathbf{r},\theta,t) - D_{\mathrm{R}}\partial_\theta^2\psi(\mathbf{r},\theta,t) = \partial_\theta\mathcal{I}_{\mathrm{int}}(\mathbf{r},\theta,t) \tag{34}$$

For interaction-free particles moving in a homogeneous media, the r.h.s of the above equation would vanish. $\psi$ would be merely advected due to self-propulsion, and would diffuse in the $\theta$ direction due to angular noise. The angular current $\mathcal{J}_{\mathrm{int}}$ accounts for the roller-roller interactions. Starting from the microscopic equations of motion, Eqs. (24) and (25), we derived the functional form of $\mathcal{J}_{\mathrm{int}}(\mathbf{r},\theta,t)$ in [1]. In brief, as the range of the effective potential $\mathcal{H}$ is of the order of 40 colloid radii, even at the lowest colloid fraction, each particle interacts on average with $\sim 200$ neighbors. This large number suggests using a mean-field description to establish the functional form of $\mathcal{J}_{\mathrm{int}}$. We therefore assume that the two-point function factorizes as: $\psi^{(2)}(\mathbf{r},\theta;\mathbf{r}',\theta') = \psi(\mathbf{r},\theta)\psi(\mathbf{r}',\theta')$ and vanishes for $|\mathbf{r}-\mathbf{r}'| < 2a$, in order to account for the finite size of the rollers. $\mathcal{J}_{\mathrm{int}}$ then takes the form:

$$\mathcal{J}_{\mathrm{int}} = -\psi(\mathbf{r},\theta)\int_{|\mathbf{r}-\mathbf{r}'|>2a} \mathrm{d}\theta'\mathrm{d}\mathbf{r}'\psi(\mathbf{r}',\theta')\partial_\theta\mathcal{H}(\mathbf{r}-\mathbf{r}';\theta,\theta') \tag{35}$$

Integrating the above equation over $\theta$, we recover the mass conservation relation:

$$\partial_t\rho(\mathbf{r},t) + \nabla\cdot\mathbf{J}(\mathbf{r},t) = 0, \tag{36}$$

where the roller current $\mathbf{J}(\mathbf{r},t)$ and velocity fields are defined as $\mathbf{J} \equiv \nu_0\int\mathrm{d}\theta\,\hat{\boldsymbol{\nu}}\psi(\mathbf{r},\theta,t)$, and $\mathbf{J} \equiv \rho\mathbf{v}$. The dynamical evolution of $\mathbf{J}(\mathbf{r},t)$ is obtained by multiplying Eq. 34 by $\hat{\mathbf{v}}$ and integrating it over the angular variable. At leading order in a systematic gradient expansion it takes the form:

$$\begin{aligned}\partial_t\mathbf{J} + v_0^2\nabla\cdot\left[\rho\left(\mathbf{Q}+\frac{1}{2}\mathbb{I}\right)\right] =& -D_{\mathrm{R}}\mathbf{J} + \alpha_1\rho(\mathbb{I}-2\mathbf{Q})\cdot\mathbf{J} - \beta\frac{v_0}{2}(\mathbb{I}-2\mathbf{Q})\cdot\rho\nabla\rho \\ &+ \alpha_2\rho(\mathbb{I}-2\mathbf{Q})\cdot\Delta\mathbf{J} + \gamma_2\rho(\mathbb{I}-2\mathbf{Q})\cdot\tilde{\Delta}\mathbf{J},\end{aligned} \tag{37}$$

where

$$\tilde{\Delta} = \begin{pmatrix}\partial_{xx}-\partial_{yy} & 2\partial_{xy}\\ 2\partial_{xy} & \partial_{yy}-\partial_{xx}\end{pmatrix}, \tag{38}$$

and where $\alpha_1 = 0.5\,\tau^{-1}$ and the elastic constant $\alpha_2 = \frac{Ha}{7}\tau^{-1}$ stem for the velocity-alignment interactions at the microscopic level ($A$ terms in Eq. (25)). $\beta = \frac{a}{2}\tau^{-1}$ originates from the repulsive interactions ($B$ terms in Eq. (25)).

finally the anisotropic elasticity constant $\gamma_2$ results from the $C$ terms in Eq. (25) which couple the roller orientations and relative positions.

At this stage, we do not have a closed set of hydrodynamic equations but only a relation between $\rho$, $\mathbf{J}$ and the local nematic tensor $\mathbf{Q}$, defined as: $\rho\mathbf{Q} = \langle\hat{\boldsymbol{\nu}}\hat{\boldsymbol{\nu}} - \frac{1}{2}\mathbb{I}\rangle$. An additional closure relation is required to establish the hydrodynamic theory of this active material.

### *6.3 . Hydrodynamic theory*

Deep in the polar-liquid phase we assume Gaussian fluctuations of the velocity field. This ansatz imposes the relation

$$\mathbb{Q} = \frac{1}{\nu_0^6} v^4 \left(\mathbf{v}\mathbf{v} - \frac{\nu_0^2}{2}\mathbb{I}\right). \tag{39}$$

Using this relation in Eq. (37) we find the hydrodynamic equation of the polar liquid formed by interacting colloidal rollers. Once linearized around a homogeneous flow field $\mathbf{v} = (u_0 + u)\hat{\mathbf{x}} + v\hat{\mathbf{y}}$ it takes the very same form as the linearized Toner and Tu equations:

$$\partial_t\rho + \rho_0\partial_y v + u_0\partial_x\rho = D'\partial_x^2\rho \tag{40}$$

$$\partial_t v + \lambda_1 u_0\partial_x v = -\sigma\partial_y\rho + D_\perp\partial_y^2 v + D_\parallel\partial_x^2 v + u_0 D_\rho\partial_{xy}^2\rho \tag{41}$$

where all the hydrodynamic coefficients are now defined from the microscopic interaction parameters:

$$\lambda_1 = \frac{u_0^2}{\nu_0^2} \tag{42}$$

$$\sigma = \frac{a^2}{2\tau}u_0(\rho_0) \tag{43}$$

$$D_\perp = \frac{5Ha\rho_0}{14\tau} \tag{44}$$

$$D_\parallel = \frac{3Ha\rho_0}{14\tau} \tag{45}$$

$$D_\rho = \frac{D_\perp - D_\parallel}{\rho_0} \tag{46}$$

$$D' = 0 \tag{47}$$

Eqs. (40) to (47) fully prescribe the linear hydrodynamic equations of colloidal-roller liquids. Several comments are in order. All material constants depend on the liquid density. However deep in the polar phase the polar liquid flows at a speed indistinguishable from the individual roller speed $\nu_0$ and $\lambda_1 \sim$ constant. $D'$ is vanishingly small in agreement with our experimental measurements. $D'$ is indeed measured to be 4 orders of magnitude smaller than all the other elastic constants, see Fig. 3. $D_\perp$, $D_\parallel$ and $D_\rho$ are related by Eq. (46). The value of $D_\parallel$, which we cannot measure directly, can thus be inferred from $D_\perp$ and $D_\rho$

These predictions are confronted to our spectroscopy method in Figure 3 in the main document and validate the relevance of active-sound spectroscopy to infer the material constants of broken-symmetry active materials from their fluctuation spectra.

### *6.4 . Critical discussion of the kinetic theory*

We highlight in this section the numerous assumptions required to derive the hydrodynamic equations for the colloidal-roller liquid starting from the microscopic description of the Quincke phenomenon, at the single-colloid level [1]. Despite these numerous approximations the convective coefficient ($\lambda_1$), and the compressibility ($\sigma$) of the active fluid are correctly predicted. The elastic constants are however overestimated. Kinetic theory only provides the correct orders of magnitude and more importantly their variations with $\rho_0$. A better theory should address the following issues:

1. *Quincke rotation near a conducting wall.* Our description of the Quincke mechanism is classically performed in the limit of vanishingly small Debye length. This approximation might be too severe when, as in our experiments, the colloids lie on a charged surface.

2. *Orientational interactions.* When describing the interactions between Quincke rollers, we neglect the interaction forces, and focus on the interactions torques. Simply put we assume the roller velocity $\nu_0$ to be a constant, and the roller velocity to be slaved to their orientation. This approximation is theoretically justified by the fact that the Quincke mechanism results from a spontaneous symmetry breaking. Therefore, the single-colloid orientation is slaved to a soft-mode. In practice, we do observe fluctuations of $\nu_0$ of the order of $10\,\%$. An improved theory should take into account the interaction forces as well.

3. *Far-field interactions.* The disturbances to the electric and hydrodynamic fields induced by the rollers were computed in the far-field limit. The resulting interactions are therefore an approximate of the actual interactions which also include near-field contributions.

4. *Interaction range.* Both the hydrodynamic and electric field induced by the roller motion are exponentially screened over a distance of the order of the channel height $H$. In our theory we approximate this screening by a step function.

5. *Mean-field approximation in the kinetic theory.* Another severe approximation is the mean-field assumption used to factorize the two-point function as $\psi^{(2)}(\mathbf{r},\theta,t;\mathbf{r}',\theta',t) = \psi(\mathbf{r},\theta,t)\psi(\mathbf{r}',\theta',t)$. This approximation is especially questionable deep in the ordered phase where we do observe local structural correlations.

6. *Gaussian approximation.* In order to close the hierarchy of equations for all the angular moments of $\psi$, we had to resort to a Gaussian approximation for the angular fluctuations of the roller orientation.

These approximations are numerous, and some are uncontrolled. The fair agreement with our measurements points toward a remarkable robustness of this simplified model. Going beyond these approximations is a significant challenge for active matte theorists.

## SUPPLEMENTARY NOTE 3 : INDEPENDENCE OF THE MATERIAL PARAMETERS ON THE CHANNEL GEOMETRY

In order to ascertain that the material parameters measured by active-sound spectroscopy correspond to bulk properties. We conducted a series of two experiments in microfluidc channels of width 1 mm and 2 mm. Figs. 4a and 4a indicates that the velocity fluctuation spectra are not altered by confinement. Accordingly, the angular variations of the speed of sound measured in the two channels are indistinguishables within our experimental accuracy. Fitting the speed of sound with the Toner Tu prediction gives $\lambda_1 = 0.75 \pm 0.1$ and $\sigma = 1.1 \pm 0.1\,(\mathrm{mm/s})^2$. All measurements reported in the main text correspond to experiments performed in 2 mm-wide channels and therefore correspond to bulk properties.

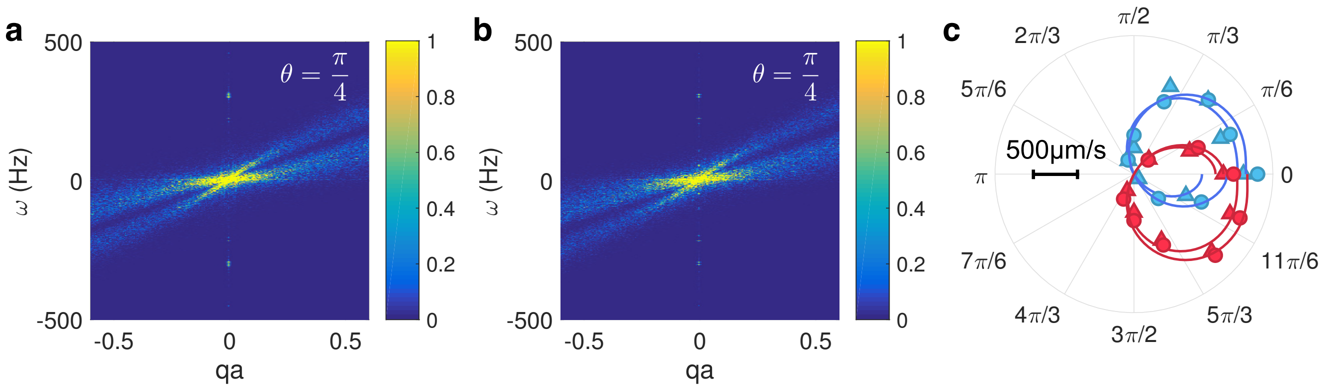


Supplementary Figure 4. **Impact of confinement on sound propagation** **a**, Power spectrum of the transverse velocity fluctuations $\langle|v_{q,\omega}|^2\rangle/\langle|v_{q=0,\omega=0}|^2\rangle$, in a channel of width 1 mm. $\theta = \pi/4$ and $\rho_0 = 0.06$. **b**, Power spectrum of the transverse velocity fluctuations $\langle|v_{q,\omega}|^2\rangle/\langle|v_{q=0,\omega=0}|^2\rangle$, in a channel of width 2 mm. $\theta = \pi/4$ and $\rho_0 = 0.07$. **c**, Polar plots of the speed of sound, $c_{\pm}(\theta) = \lim_{q\to 0}[\omega \pm (\theta)/q]$ measured from the slope at $q = 0$ of the dispersion relations. Experimental data: dots (1 mm wide channel), triangles (2 mm wide channel). Solid lines: theoretical fits. Same experimental conditions as in **a** and **b**.

## EXPERIMENTAL SETUP

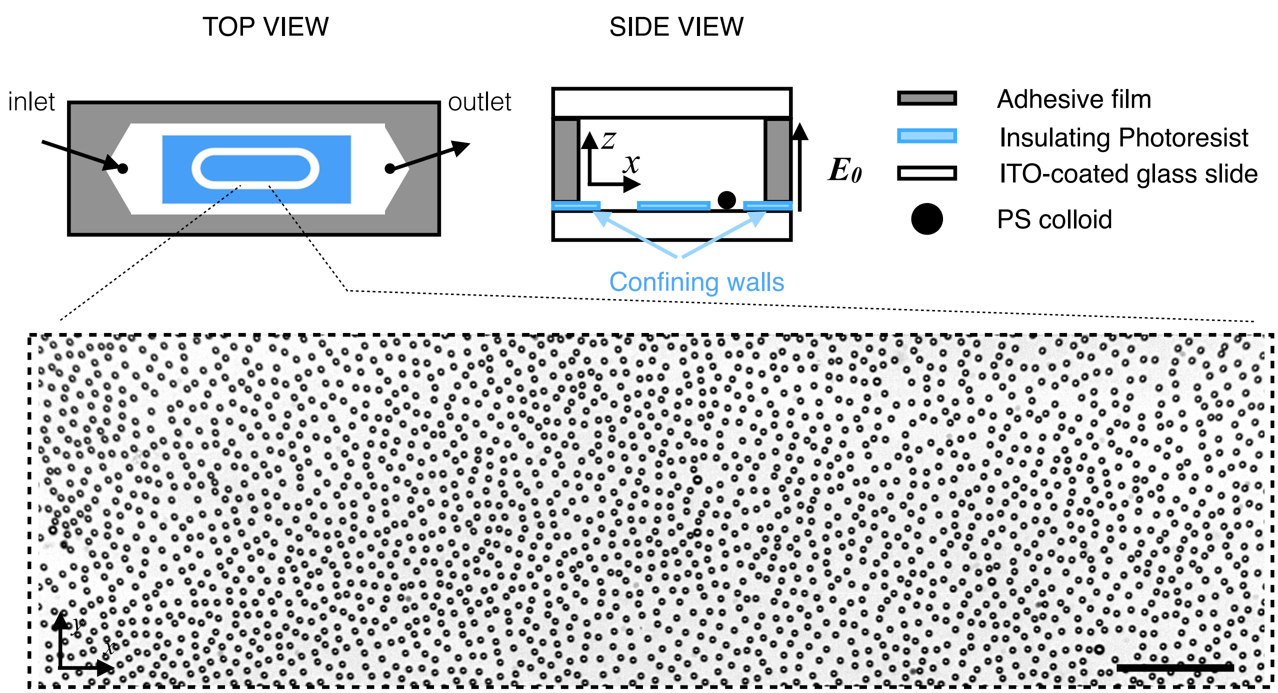


Supplementary Figure 5. **Sketch of the microfluidic device. Top view.** A one-centimeter wide channel is used to flow the PS colloids. A pattern in the shape of a racetrack confines the rollers. The picture shows a snapshot of a polar liquid flowing along the racetrack. Scale bar: 100 $\mu$m. The observation window shows only a small part of the colloidal liquid. **Side view.** The colloids roll on the bottom electrode, the obstacles electrostatically repel the rollers. An adhesive film (double-sided scotch tape) sets the gap between the electrodes.

## SUPPLEMENTARY REFERENCES


[1] Antoine Bricard, Jean-Baptiste Caussin, Nicolas Desreumaux, Olivier Dauchot, and Denis Bartolo, "Emergence of macroscopic directed motion in populations of motile colloids," Nature **503** (2013).

[2] Alexandre Morin, Nicolas Desreumaux, Jean-Baptiste Caussin, and Denis Bartolo, "Distortion and destruction of colloidal flocks in disordered environments," Nature Physics **1**, 1–6 (2016).

[3] John Toner and Yuhai Tu, "Long-range order in a two-dimensional dynamical XY model: How birds fly together," Phys. Rev. Lett. **75**, 4326–4329 (1995).

[4] John Toner, Yuhai Tu, and Sriram Ramaswamy, "Hydrodynamics and phases of flocks," Annals of Physics **318**, 170 – 244 (2005), special Issue.

[5] M. C. Marchetti, J. F. Joanny, S. Ramaswamy, T. B. Liverpool, J. Prost, Madan Rao, and R. Aditi Simha, "Hydrodynamics of soft active matter," Rev. Mod. Phys. **85**, 1143–1189 (2013).

[6] E. Bertin, M. Droz, and G. Grégoire, "Hydrodynamic equations for self-propelled particles: microscopic derivation and stability analysis," Journal of Physics A: Mathematical and Theoretical **42**, 445001 (2009).

[7] F. D. C. Farrell, M. C. Marchetti, D. Marenduzzo, and J. Tailleur, "Pattern formation in self-propelled particles with density-dependent motility," Phys. Rev. Lett. **108**, 248101 (2012).

[8] J.-B. Caussin and D. Bartolo, "Tailoring the interactions between self-propelled bodies," The European Physical Journal E **37**, 55 (2014).

[9] J. R. Melcher and G. I. Taylor, "Electrohydrodynamics: A review of the role of interfacial shear stresses," Annual Review of Fluid Mechanics **1**, 111–146 (1969).

[10] Antoine Bricard, Jean-Baptiste Caussin, Debasish Das, Charles Savoie, Vijayakumar Chikkadi, Kyohei Shitara, Oleksandr Chepizhko, Fernando Peruani, David Saintillan, and Denis Bartolo, "Emergent vortices in populations of colloidal rollers," Nature communications **6** (2015).

[11] Daiki Nishiguchi, Ken H. Nagai, Hugues Chaté, and Masaki Sano, "Long-range nematic order and anomalous fluctuations in suspensions of swimming filamentous bacteria," Phys. Rev. E **95**, 020601 (2017).
